# Supplementary material for: EnVisionVR: A Scene Interpretation Tool for Visual Accessibility in Virtual Reality
Source: arXiv:2502.03564 source file (2025-02-05)
Supplement: Supplementary file 1 [file evr-study-questionnaire.pdf]

# Practice Scene

I'm going to ask you to rate a statement, telling me if you think it is likely or unlikely it is to be correct. A 'low' score of 1 says you think the statement is very *\*un\**likely to be correct, and a 'high' score of 5 says you think the statement is very likely to be correct. Are you ready for the statement? <read statement>

Okay, how likely is that statement to be correct, on a scale of 1 to 5?

1. You are situated in a kitchen.

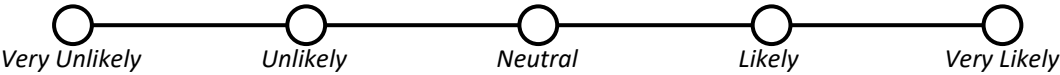

2. Please orient yourself so that you are facing towards the couch.

Task Completed? (Y/N):

3. Please use the controller to pick up the mug on the white coffee table.

Task Completed? (Y/N):

# Test Scene

I'm going to ask you to rate a statement, telling me if you think it is likely or unlikely it is to be correct. A 'low' score of 1 says you think the statement is very \*un\*likely to be correct, and a 'high' score of 5 says you think the statement is very likely to be correct. Are you ready for the statement? <read statement>

Okay, how likely is that statement to be correct, on a scale of 1 to 5?

If Anchor 1: This is a scene of a classroom with a desk and a chair.

If Anchor 2: There is a shelf filled with various objects beside the cauldron.

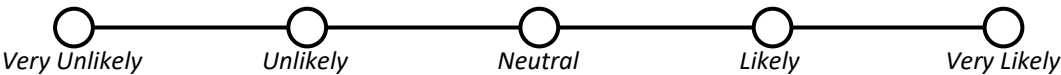

At this point I'd like you to turn and face an object in the room.

If Anchor 1: Turn to face the radio.

If Anchor 2: Turn to face the kitchen counter.

Task Completed? (Y/N):

At this point I'd like you to interact with an object in the room.

If Anchor 1: Pick up the golden key on the desk.

If Anchor 2: Please press the "Brew" button on the control panel in front of the cauldron.

Task Completed? (Y/N):

1a. How easy (or not) was it to understand the scene?

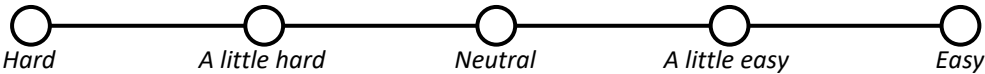

1b. How easy (or not) was it to face towards particular virtual objects within the scene?

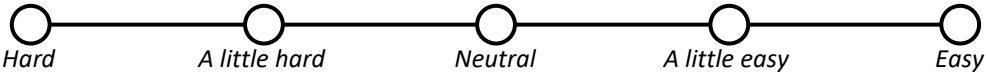

1c. How easy (or not) was it for you to interact with the scene?

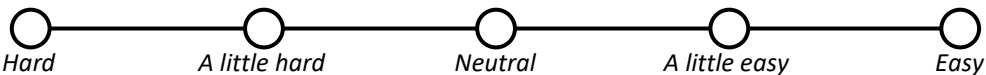

# Post-Study Interview

## Overall Experience

Which of the two conditions did you find most helpful? (EnVisionVR or No-Assistance)

## Do you have any comments/suggestions for this accessibility tool?

For EnVisionVR, which accessibility features did you find helpful (Where am I / What is near me / Where is the <object name>)? Why?

Is there anything missing from the tools that would have helped you?

What particular requirements do you have for a VR accessibility system given what your blindness or visual impairment means for your experience of VR? ?
